# Supplementary material for: Spin models inferred from patient data faithfully describe HIV fitness landscapes and enable rational vaccine design
Source: arXiv:1306.2029 source file (2013-06-09)
Supplement: Supplementary file 1 [file shekhar_fitness_SI.pdf]

# Supporting Information for Shekhar et. al.

## 1 Sampling $H_{int}[\vec{s}]$ and low dimensional representation using PCA

Let $\vec{s^n} \in \{0,1\}^{1\text{x}N}$ be an arbitrary sequence[1] in an equilibrium ensemble of $\mathcal{M}$ sequences sampled according to $H_{int}[\vec{s}]$ using the Metropolis Monte Carlo (MC) algorithm[1]. This ensemble is comprised of sequences from six independent realizations of $10^8$ steps each, where each step constitutes an attempt to flip a single site. We eliminated the first $10^4$ steps for equilibration, and recorded every $i^{th}$ state such that $mod(i, 5N) = 0$. The sequences in the MC ensemble (also referred to as "equilibrium ensemble") capture the statistical properties of the intrinsic fitness landscape as encoded by $H_{int}[\vec{s}]$. The "mean sequence" of the MC ensemble is defined as,

$$\vec{s^{av}} = \frac{1}{\mathcal{M}} \sum_{n=1}^{\mathcal{M}} \vec{s^n} \tag{S1}$$

Here, $\vec{s^{av}} \in \mathbb{R}^{1\text{x}N}$. The sample covariance matrix $\mathbf{C} \in \mathbb{R}^{N\text{x}N}$ is defined as,

$$\mathbf{C}_{ij} = \frac{1}{\mathcal{M}} \sum_{n=1}^{\mathcal{M}} \left(s_i^n - s_i^{av}\right)\left(s_j^n - s_j^{av}\right) \tag{S2}$$

Principal component analysis (PCA) is a linear dimensionality reduction/ visualization technique that seeks to find a subspace comprised of fewer dimensions within the original, high dimensional feature space such that the projected variance in the new subspace is maximized. The reader

[1]Note that $N = 132$ for p17

is referred to refs. [2] and [3] for standard formulations of PCA and mathematical details. The new subspace is typically defined by few orthogonal unit vectors $\vec{u^i}$ ($i = 1, 2, 3, \ldots k$ and $k \ll N$ ), each of which is a linear combination of the orthonormal basis vectors defining the original feature space. In our problem, the latter are unit vectors in $\mathbb{R}^N$. It can be shown that the "principal directions" $\vec{u^i} \in \mathbb{R}^{N\text{x}1}$ ($i = 1\,, 2\,, 3, \ldots k$) are eigenvectors of $\mathbf{C}$ corresponding to the $k$ largest eigenvalues $\lambda_i$ ($i = 1\,, 2\,, 3, \ldots k$).

The amount of variance captured by $\vec{u^i}$ can be straightforwardly estimated as $\left(\vec{u^i}\right)^T \mathbf{C}\vec{u^i} = \lambda_i$. Consequently, the fraction of variance captured by principal direction $\vec{u^i}$ is $\frac{\lambda_i}{\sum_{j=1}^{N} \lambda_j}$. For an arbitrary sequence $\vec{s}$, its projections on to the principal directions are referred to as its "principal components" or PCs. Thus, $PC_1[\vec{s}] = \vec{s}.\vec{u^1}$, $PC_2[\vec{s}] = \vec{s}.\vec{u^2}$ and so on. The number of principal directions $k$ necessary for an effective low dimensional description of the dataset is determined heuristically by examining the eigenvalue spectrum of $\mathbf{C}$ for a "spectral gap", when $\lambda_i$ are arranged in a descending order (cf. Fig. S1). We use the first two principal components $PC_1$ and $PC_2$ to visualize the evolution of viral strains in our quasispecies simulations. Cumulatively, the top two modes capture about 30% of the variance in the data represented by the MC sampling. This may be due to the fact that the underlying geometry of the fitness landscape is highly non-linear. PCA approximates the underlying manifold as a linear combination of hyperplanes. When the underlying manifold is highly non-linear, it is known that PCA overestimates the effective dimensionality[4]. Using a highly coarse grained representation through $PC_1$ and $PC_2$, however, is not a serious problem for this work because our primary purpose is visualization, not dimensionality reduction. We compute statistical quantities like mutational probabilities and correlations using the full, original representation of sequences. The following section provides evidence that $PC_1$ and $PC_2$ separate the regions of sequence space defined by subtype B.

# 2 Visualizing the Prevalence Landscape

Each $N$-bit binary sequence $\vec{s}$ in the MC ensemble can be converted into a two dimensional representation by computing its projection onto the top two principal eigenvectors, namely $[PC_1, PC_2]$.

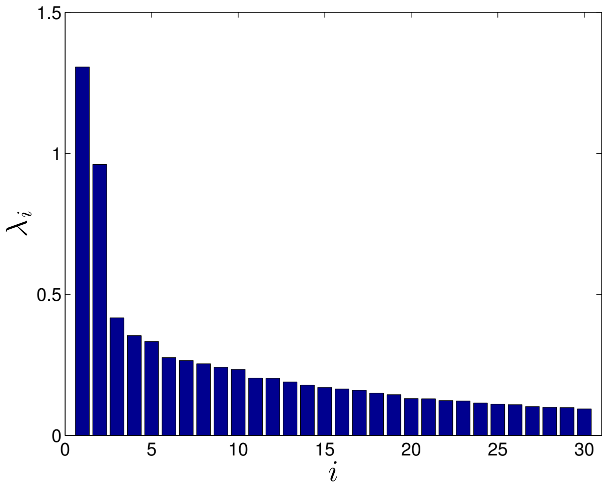


Figure S1: The top 30 eigenvalues of the covariance matrix $\mathbf{C}$ computed from the equilibrium ensemble. A spectral gap between $\lambda_2$ and $\lambda_3$ is clearly discernible.

In this manner, the embedding of every sequence in the MC ensemble was computed and used to generate probability histograms across the $[PC_1, PC_2]$-plane using a square mesh. The probabilities were converted to analogues of free energy using the statistical mechanical relation,

$$A(x, y) = -\log P(x, y) + \text{const.} \tag{S3}$$

where $A(x, y)$ is the "Helmholtz free energy" associated with the cell centered on $(x, y)$ in the $[PC_1, PC_2]$-plane and $P(x, y)$ is the sample probability of a sequence occupying this point. The free energy values were converted to contours using an in-built function in Matlab®. The resulting representation in Fig. S2 shows three fitness peaks corresponding to regions with low free energy values. Upon projecting the subtype B sequences in the MSA (black dots in Fig. S3) obtained from the Los Alamos HIV Database[5], we find that barring 3 cases (out of 2474), all the sequences are localized around a single fitness peak. These are also the sequences that were used to compute the parameters $\{J_{ij},\, h_i\}$ of $H_{int}[\vec{s}]$ in Ferguson et. al. [6]. The mutational probabilities $\langle s_i \rangle$, $\langle s_i s_j \rangle$, $\langle s_i s_j s_k \rangle$ computed from sequences generated through unrestricted sampling of $H_{int}[\vec{s}]$ do not agree with these quantities computed from the MSA containing subtype B sequences (data not shown).

As argued in Ferguson et. al. [6], the additional basins are extrapolations of the fitted non-linear model. When we restricted sampling to the primary basin around the peak corresponding to subtype B by means of reflective boundary conditions in the PC-space (Fig. S2), we find that mutational probabilities are accurately reproduced (Fig. S4). As described in the main text, excursions out of the primary basin are also restricted in the quasispecies simulations (cf. *Methods*). This is equivalent to considering excursions outside the primary basin as unfit and killing these sequences. Typical sequences in the extrapolated basins (Fig. S5 in Ref. [6]), possess a large fraction of sites that are mutated ($> 40$ %) compared to WT. In our quasispecies simulations (cf. *Methods*), escape out of the basin occurs exceedingly infrequently for mutation rates $\mu < 10^{-2}$ and thus strains are rarely killed in the *pre-screening* step.

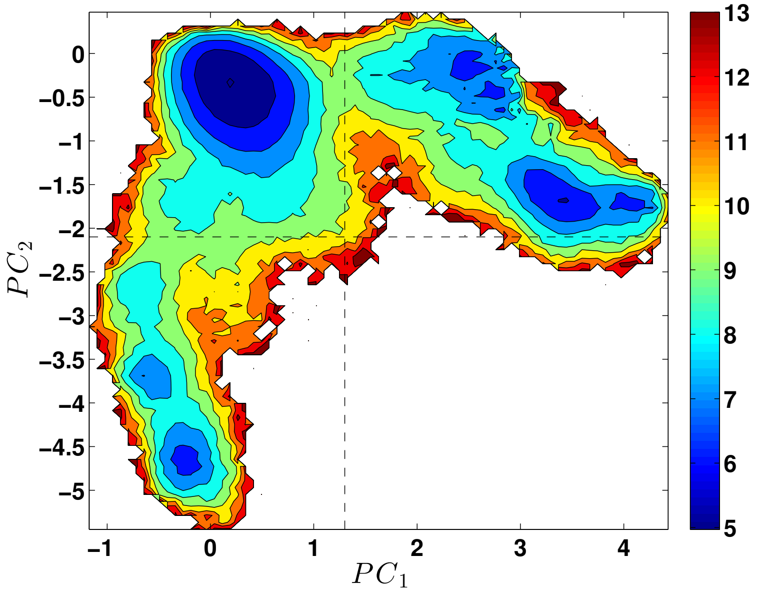


Figure S2: A lower dimensional representation of the intrinsic fitness landscape of p17 computed using principal component analysis (PCA) from sequences sampled according to $H_{int}[\vec{s}]$ using the Metropolis Monte Carlo algorithm[1]. The sequences are projected along the first two principal components (PCs) and a corresponding free energy $(A(x, y))$ map is computed according to Eq. S3. The low free energy regions correspond to high fitness states while low free energy regions correspond to unfit states in sequence space. The edges of the box in the top-left corner defined by dashed-lines are used as reflective boundaries in the quasispecies simulations. **Implementation of boundary conditions during simulation :** During the *Pre-screening* step in our intra-host simulations (cf. *Methods*), we compute $[PC_1, PC_2]$ for every sequence. Mutants that escape the box are considered unviable and deleted immediately.

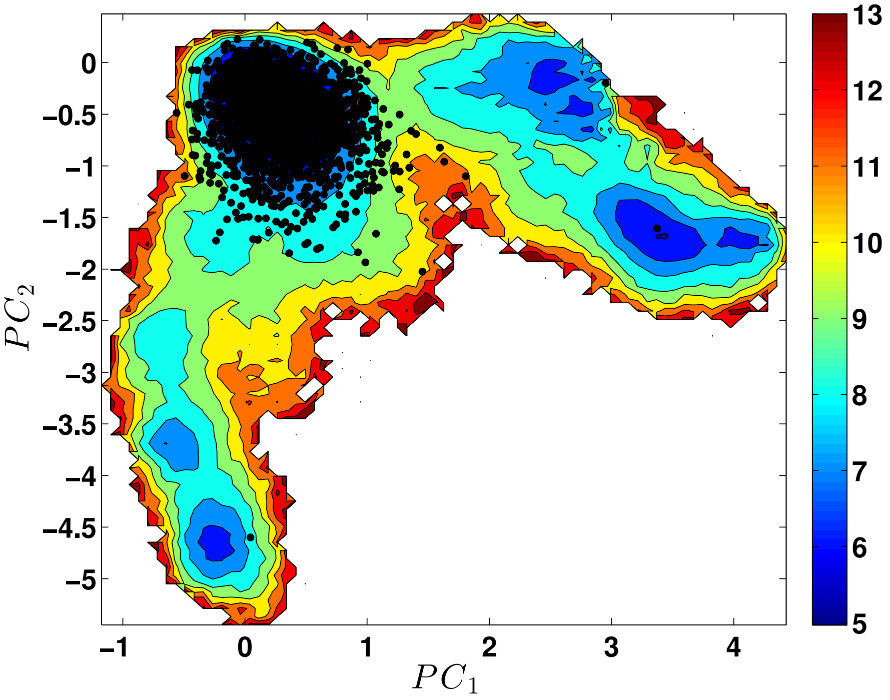


Figure S3: Subtype B sequences from the Los Alamos MSA (n=2474)[5] that were used to parametrize $H_{int}[\vec{s}]$ in ref. [6] are indicated by $\bullet$'s and are preponderantly located around one of the three fitness peaks, with the exception of three sequences.

# 3 Comparison of mutational probabilities upon restricted sampling

As stated in section 2, an unrestricted sampling of $H_{int}[\vec{s}]$ using the Metropolis algorithm results in mutational probabilities that do not agree with the corresponding quantities estimated from the MSA used to parameterize the maximum entropy model [6]. However, when we exclude from the ensemble those sequences that fall outside the upper-left "box" in $PC_1 - PC_2$ space as defined in Fig. S2, the marginals $\langle s_i \rangle_{int}$, $\langle s_i s_j \rangle_{int}$, $\langle s_i s_j s_k \rangle_{int}$ agree very well with $\langle s_i \rangle_{LANL}$, $\langle s_i s_j \rangle_{LANL}$, $\langle s_i s_j s_k \rangle_{LANL}$ (Fig. S4).

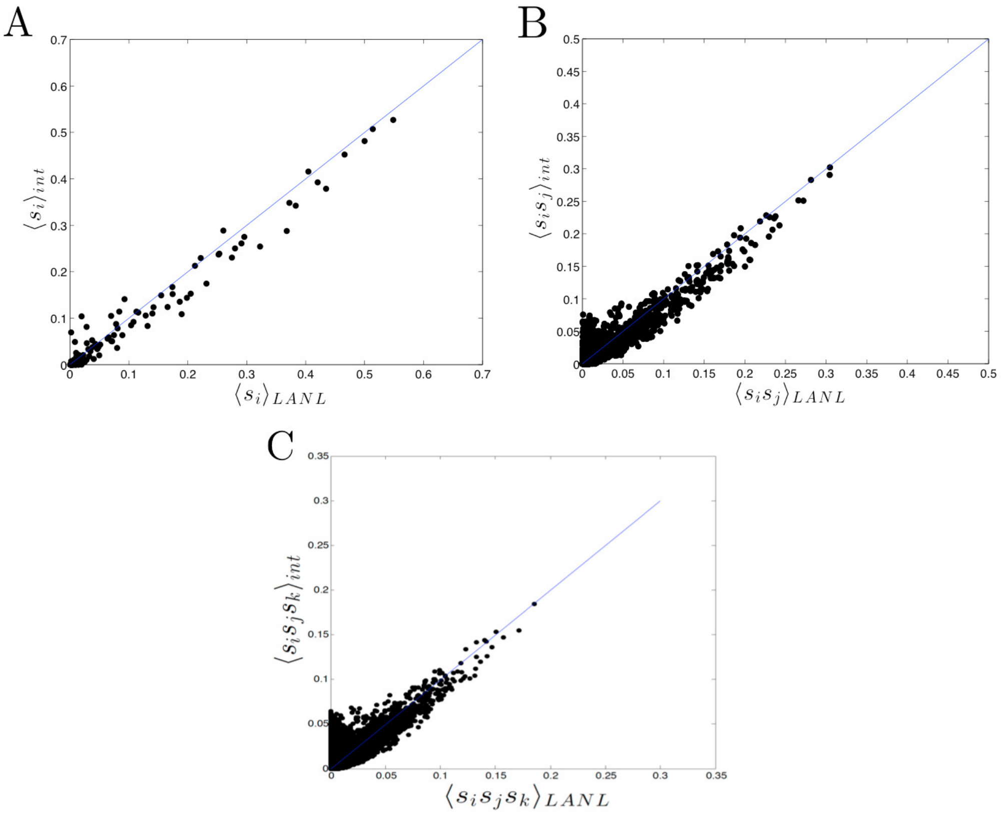


Figure S4: Comparison of the marginal one, two and three-site mutational probabilities computed from an equilibrium sampling of $H_{int}[\vec{s}]$ (y-axis) using Metropolis sampling with the corresponding values computed from the subtype B sequences obtained from the Los Alamos ($LANL$) database[5] (x-axis).

# 4 Statistics of T cell targeting of p17

We estimated the targeting frequencies of different sites in p17 within the Caucasian American population during the acute and chronic phases of HIV infection (cf. Fig. S5). In this estimate, a site is considered “targeted” if it is present in one or more epitopes (short peptides of 8-11 AA length derived from viral proteins and which are directly recognized by specific CD8 T cells during infection). While many epitopes have been clinically documented, we restricted ourselves to the most common CD8 T cell epitopes list documented by Streeck et. al.[7]. The presence of a T cell response to a particular epitope within a given individual is determined by two factors. First, the set of epitopes that are likely to be targeted by specific T cells during infection in a particular individual are determined by the specific alleles of the Human Leukocyte Antigen (HLA) gene that the individual is endowed with. These genes encode proteins that present viral epitopes to T cells, enabling the immune system to detect infection. Second, the frequency with which a particular epitope is targeted relative to others within a given HLA background is determined by the “immunodominance” of the specific T cell that recognizes the epitope[7]. For each epitope in our list, we computed the frequency of targeting by an HLA allele that binds to this epitope by combining the frequency of that allele within the Caucasian American population[8] with estimates of the epitope immunodominance[7] in each case. The overall frequency of targeting at a particular p17 site is simply a sum of the targeting frequencies of all the well-recognized epitopes that contain this site.

Of the 132 residues in p17, we find that according to our estimates, 67 are not targeted at all, 46 are targeted at a frequency than 6%, and no site is targeted by more than 23% frequency (cf. Fig. S5). In particular, we note that only 18 out of 132 p17 sites ($< 14$ %) are targeted at greater than 10% frequency in either acute or chronic phase. Strictly speaking, these estimates of the targeting frequency at each site should be regarded as lower bounds. Comprehensive epitope maps of p17 that include *all* the clinically documented epitopes have been published[9] and these suggest that every site within p17 is present in at least one documented epitope. Since most of these epitopes are targeted by alleles present in very low frequencies across the population, we do not expect their

inclusion to change the qualitative picture of T cell targeting painted by our rough estimates - that is, on average, a particular site is targeted by a small fraction of individuals in a population.

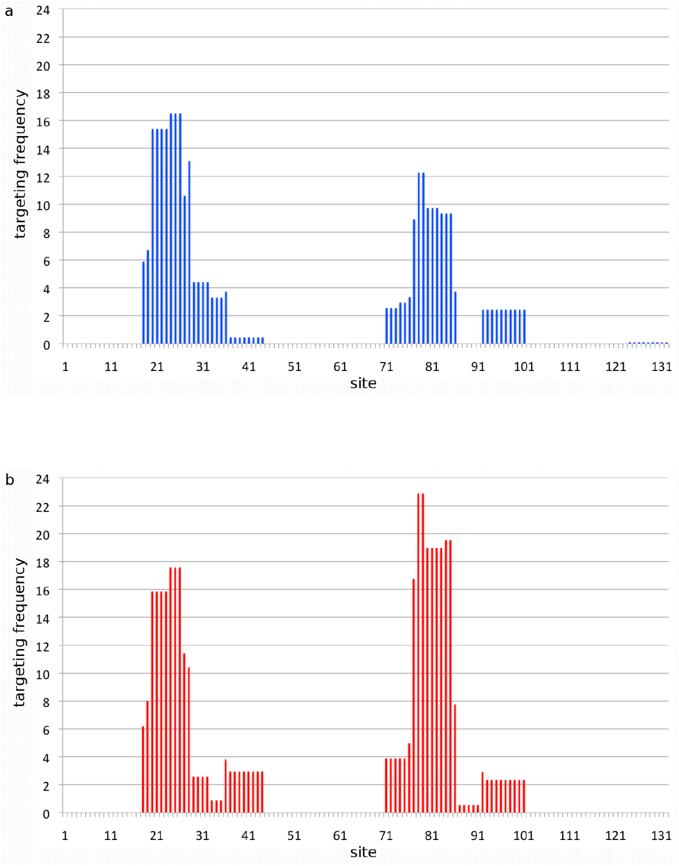


Figure S5: An estimate of the frequencies with which each residue in p17 is targeted by T cell pressure during the (a) acute phase and (b) chronic phase by HLA alleles in a general population. These estimates were computed assuming that the distribution of Human Leukocyte Antigen (genes that determine the T cell immune response in an individual) alleles follow that of the Caucasian American population[8], and combining these with the frequencies with which the most common T cell epitopes (short viral protein fragments that are directly recognized by T cells) are recognized during the acute/chronic phase across the population[7]. Actual targeting frequencies may vary due to the targeting frequency of T cell peptides for which such data is yet unavailable and stochastic variation of the immune response within particular individuals.

# 5 Robustness studies

How robust are our main results to variations in the simulation parameters, namely, the mutation rate $\mu$, the choice of parameters for the distribution generating the immune fields $\{b_i\}$, the average number of viral generations in an host $\langle \tau_S \rangle$, and the targeting intensity determined by $n_{max}$? In each case, we examined the effect of changing the parameter on the one, two and three-body mutational probabilities computed from the dynamical simulations vis-á-vis the corresponding quantities computed from the intrinsic fitness landscape. We also examined how the Spearman rank correlation between the effective fitness $H_T$ and the intrinsic fitness $H_{int}$ is affected (cf. Fig. 4).

## 5.1 The mutation rate $\mu$

Keeping all else fixed, we ran our simulations for various values of the mutation rate $\mu$ in the range $10^{-5}$ to 0.5. We repeated these simulations for different choices of the distributions that generated the $\{b_i\}$ fields with similar results, but the trends we describe here are for the base case of a Gaussian distribution with mean and variance equal to the sample mean and variance of the $\{h_i\}$ fields, as introduced in the main text. At very low mutation rates ($\mu < 10^{-4}$), we find that the one, two and three-body mutational probabilities computed from the population ensemble ($\langle s_i \rangle_{dyn}$, $\langle s_i s_j \rangle_{dyn}$ and $\langle s_i s_j s_k \rangle_{dyn}$) are close to zero (Fig. 3a, c). Mutations are rarely sampled in this regime, and the quasispecies in different hosts remain localized around the WT strain in the fitness landscape (cf. Fig S8).

At intermediate values of $\mu \in (10^{-4}, 10^{-2})$, the agreement between the mutational probabilities reflected by the dynamics and those computed from equilibrium sampling of the intrinsic fitness landscape improves. This is also reflected in the rank correlation between $H_T$ and $H_{int}$ for subtype B sequences which increases from 0.72 to 0.9 as $\mu$ increases from $5 \times 10^{-4}$ to $10^{-2}$ (cf. Fig S6a-c). At high mutation rates $\mu > 10^{-2}$, however, mutations rapidly accumulate in the quasispecies in every generation. The accumulation of a large number of mutations ($> 20$) increases the likelihood of elimination in the *Pre-Screening* step (cf. *Methods*) if the strain escapes the basin defined by subtype B sequences. Possession of a large number of mutations also increases the chance of deleterious

combination of mutations (high $J_{ij}$), which can lead to deletion of such strains in the *Selection* step (cf. *Methods*). The strains that survive these steps and prevail in the population ensemble possess a large number of mutations, and the mutational probabilities $\langle s_i \rangle_{dyn}$, $\langle s_i s_j \rangle_{dyn}$ reflected by these sequences overestimate their counterparts estimated from intrinsic fitness alone.

At high mutation rates, the rapid accumulation of deleterious mutations can lead to the death of all strains in the quasispecies in some hosts. We regard such cases as unsuccessful infections and these hosts are discarded from the simulation. Only hosts where the quasispecies is viable are considered "productively infected" and are sampled for the consensus sequence, which is added to the population ensemble. As $\mu$ increases, the number of successfully infected patients decreases. For e.g., in all the simulations between $\mu = 10^{-4}$ to $\mu = 10^{-2}$, the number of viable consensus sequences were in the range 4700-5500, suggesting that approximately 70-90% of the patients in our simulation were successfully infected such that the quasispecies within these patients had achieved a mutation-selection balance and was stable. In contrast at $\mu = 0.05$, $\mu = 0.1$ and $\mu = 0.3$ this number decreased to 1983 (30% of the total patients), 334 (5% of the total patients), and 0 respectively. This is related to the phenomenon of error catastrophe proposed by M. Eigen [10] but we hasten to qualify that in our finite system, the transition is not a sharp one as has been demonstrated for Eigen's model under certain kinds of fitness landscapes in the infinite population limit. The sharpness of the transition may also be attenuated by the finite size effects due to small effective population sizes we have considered and the length of our protein. That these parameters play a role has been demonstrated in the case of simpler fitness landscapes through stochastic simulations [11].

Taken together, our results in this section suggest that there is an intermediate range of mutation rates where immune selection leads to an efficient exploration of the fitness landscape preserving its correlation structure in the population ensemble.

## 5.2 Varying parameters of the Gaussian distribution generating $\{b_i\}$

We varied the mean $s_h$ of the Gaussian distribution from which the immune parameters $\{b_i\}$ were sampled, while keeping the variance of the distribution fixed to $\sigma_h^2$ (the sample variance of the

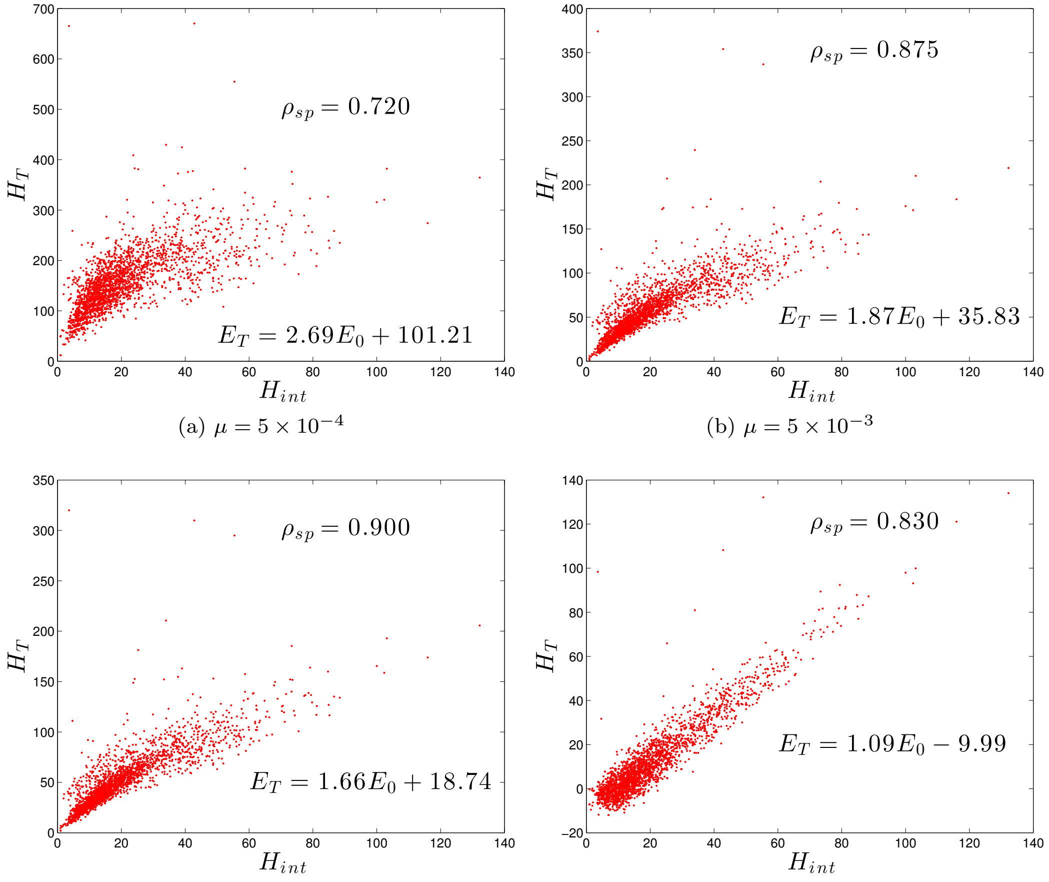


(a) $\mu = 5 \times 10^{-4}$ (b) $\mu = 5 \times 10^{-3}$

(c) $\mu = 10^{-2}$ (d) $\mu = 10^{-1}$

Figure S6: Rank correlation between $H_T$ and $H_{int}$ for different mutation rates $\mu$. Here, $n_{max} = 6$ and $\{b_i\}$'s were sampled from a Gaussian distribution with mean $\bar{h}$ and variance $\sigma_h^2$.

fitted $\{h_i\}$ values). For the value of the mean, we used $0.2\bar{h}$, $0.5\bar{h}$, $\bar{h}$, $2\bar{h}$, $5\bar{h}$, and $10\bar{h}$ where $\bar{h}$ is the sample mean of $\{h_i\}$ and also the canonical value of $s_h$ as introduced in the main text. The rate of mutation $\mu$ was fixed at the value $5 \times 10^{-3}$. We found that the correlation coefficient between the effective and intrinsic energies, namely $H_T$ and $H_{int}$, varied non-monotonically with $s_h$. While the rank correlation coefficient increased from 0.85 to 0.9 as $s_h$ increased from $0.2\bar{h}$ to $2\bar{h}$, it decreased to 0.78 and 0.47 for $5\bar{h}$ and $10\bar{h}$, respectively (cf. Fig S7). At low and high values of $s_h$, the agreement was poor between the one, two and three-body mutational probabilities (data not shown). At low values, the immune pressure is negligible and the quasispecies in different individuals remains localized around the WT sequence. In the mean-field approximation to $H_T$ (Eq. 6, main text), $\bar{b_i} \approx 0$ and the field at each site is offset from its equilibrium value by the ferromagnetic term arising from the mutational coupling between generations. At very high values of $s_h$, mutations are immediately selected at sites subjected to immune pressure irrespective of their intrinsic propensity (based on $h_i$'s and $J_{ij}$'s). Thus the mutational probabilities at the population level become enslaved to the statistics of immune pressure at that site and no longer pay heed to the constraints at intrinsic fitness, resulting in poor correlation between $H_T$ and $H_{int}$. At intermediate values of $s_h$, the mutational probabilities and the effective energies correlated with their intrinsic counterparts. For all of these simulations, the number of viable sequences were in the range 4500 to 5500.

### 5.3 Uniform distribution

We sampled $\{b_i\}$ according to a uniform distribution between the minimum and the maximum among the $\{h_i\}$ values. Within this setting, varying the mutation rate $\mu$ produced results that were qualitatively similar to those reported in section 5.1 above (data not shown). Between $\mu = 5 \times 10^{-4}$ and $\mu = 10^{-2}$, the rank correlation between $H_T$ and $H_{int}$ increased from 0.63 to 0.91 and the slope of the best fit line between simulated and equilibrium energies decreased from 2.46 to 1.34, just as reported in section 5.1 for Gaussian distributed $\{b_i\}$. However, further increase in the mutation rate led to a decrease in the rank correlation coefficient. For instance, at $\mu = 0.1$, the rank correlation was 0.77 but with only 255 viable sequences ($\sim$ 3% of the total patients). The

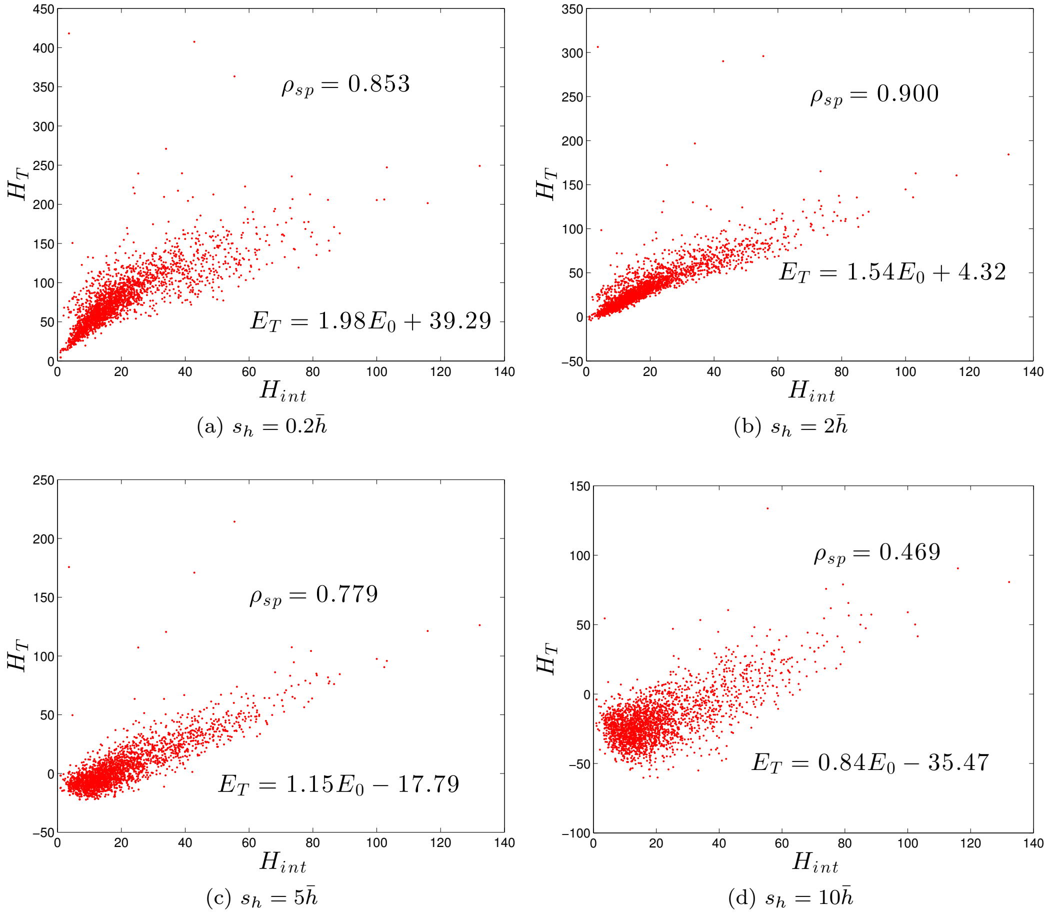


(a) $s_h = 0.2\bar{h}$

(b) $s_h = 2\bar{h}$

(c) $s_h = 5\bar{h}$

(d) $s_h = 10\bar{h}$

Figure S7: Rank correlation between $H_T$ and $H_{int}$ for different values of $s_h$. $\mu = 5 \times 10^{-3}$

number of viable sequences within the population ensemble gradually decreased beyond $\mu = 0.01$ similar to the phenomenon of error threshold. At $\mu = 0.3$, there were no viable sequences in the population ensemble, suggesting that the error threshold had been crossed.

The agreement between the simulated and the intrinsic one, two and three-body mutational probabilities also varied with the mutation rate. At very low mutation rates $\mu < 5 \times 10^{-4}$ these quantities were close to zero in the simulations, whereas at very high mutation rates $\mu > 0.05$, there were few viable sequences in the population ensemble and the prevailing sequences overestimated the mutational probabilities. At intermediate mutation rates, the mutational probabilities from the population ensemble agreed with the intrinsic values, as reported in section 5.1.

## 5.4 Number of generations

Within each host, the number of generations that the viral quasispecies evolve is a random number uniformly chosen between the limits $\tau_{min}$ and $\tau_{max}$. For our canonical simulations, we chose $\tau_{min} = 25$ and $\tau_{max} = 500$. Empirically, we noted that any $\tau_{max} \geq 275$ ($\langle \tau_S \rangle \geq 150$) did not change the qualitative nature of our results but three runs at $\tau_{max} = 150$ yielded results that were the mutational probabilities poorly correlated with their intrinsic counterparts (data not shown). The likely reason for this discrepancy is that the viral quasispecies requires a minimum number of generations to "sense" the immune pressure and make adaptive mutations. If the number of generations is "long enough" the quasispecies reaches a stationary distribution. In contrast, if the virus is sampled in a transient phase, most the mutations in its proteome might not represent the correlation structure of the fitness landscape accurately. Within our model, we expect the minimum number of generations needed to sense the immune response to be inversely correlated with $N_v$ since the emergence of a strain with a combination of mutations that perfectly adapts (low $H[\vec{s}]$) to the immune response and dominates the quasispecies increases with $N_v$.

We also ran simulations by incorporating a "wait-time" in our intra-host simulations before the immune pressure is turned on. This was implemented by fixing $b_i = 0 \; \forall \; i$ until $\tau_{min}$ generations in a new host, after which the immune pressure becomes non-zero. Simulations for $\tau_{min} = 0, 10, 15$ and 25 yielded results that were qualitatively consistent with each other.

## 5.5 Changing $n_{max}$

The parameter $n_{max}$ determines the intensity of immune targeting since any infected host is set to randomly target a number of protein residues that is chosen uniformly between 0 and $n_{max}$. As noted in the main text, our choice of $n_{max}$ to be a low number was motivated from clinical data indicating that any given person is predisposed by her/his genetic makeup to target few sites within viral proteins [6]. The results we report in the main text are for $n_{max} = 6$. These remain qualitatively consistent up to $n_{max} = 20$ but for higher values ($n_{max} = 30, 35$ and 50), the agreement between the mutational probabilities (and consequently energies) started deteriorating. As $n_{max}$ increases, the mutational probabilities estimated from the population ensemble overestimate the the corresponding values computed from sampling $H_{int}$. When $n_{max}$ is large, the immune response is no longer perturbative in that a large fraction of the population targets every site on the protein leading to the statistics of mutations at these sites being governed by “immune footprints”.

## 6 Visualizing quasispecies diversity in the absence and presence of immune pressure

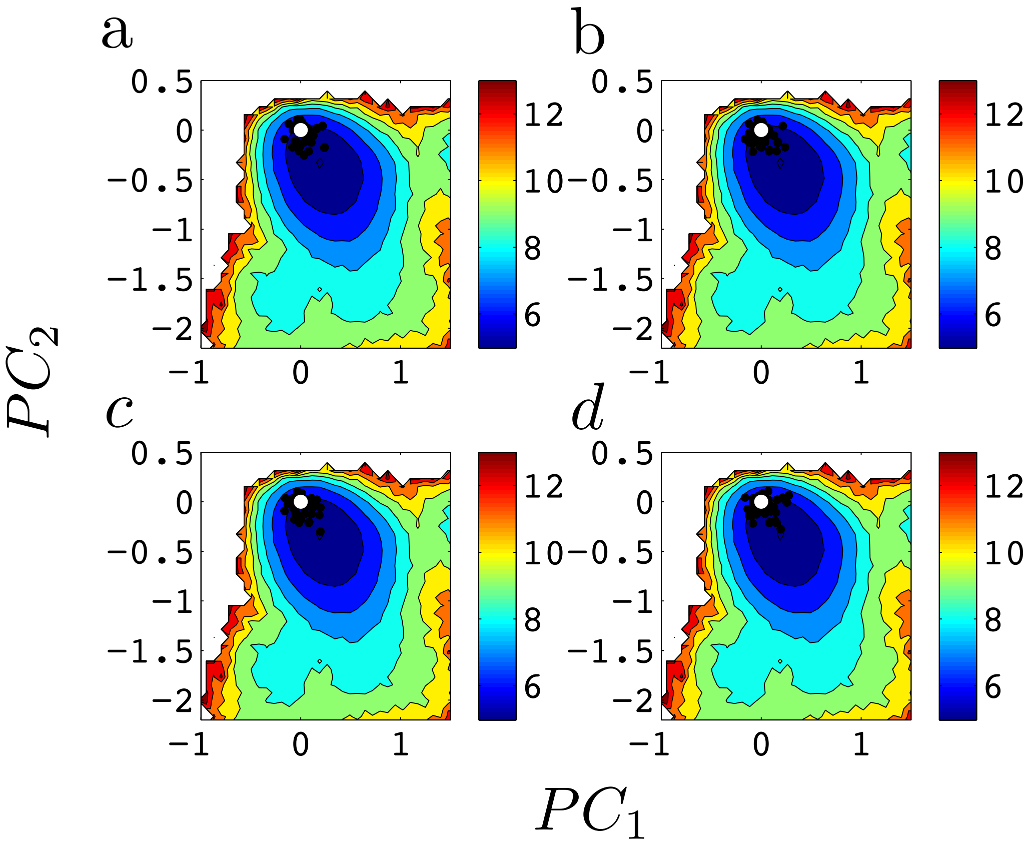


Figure S8: Panels a-d depict viral quasispecies in four randomly chosen individuals in the absence of immune pressure ($\vec{b} = 0$ in all hosts). Every unique strain within the quasispecies is represented by a black dot at its location on the landscape. As can be readily discerned, different individuals have very similar quasispecies, where the constituent mutant strains are localized around the WT strain $\vec{s} = \vec{0}$ in sequence space (which corresponds to the point $(PC_1, PC_2) = (0, 0)$). In the absence of an external selective force in the form of immune pressure, mutations that are deleterious to viral fitness are not selected at the population level, although they do transiently appear within the quasispecies of individual infected hosts. The WT strain is always the dominant strain within individual quasispecies (represented by a white dot) and consequently, the population ensemble in these simulations is exclusively comprised of WT strains.

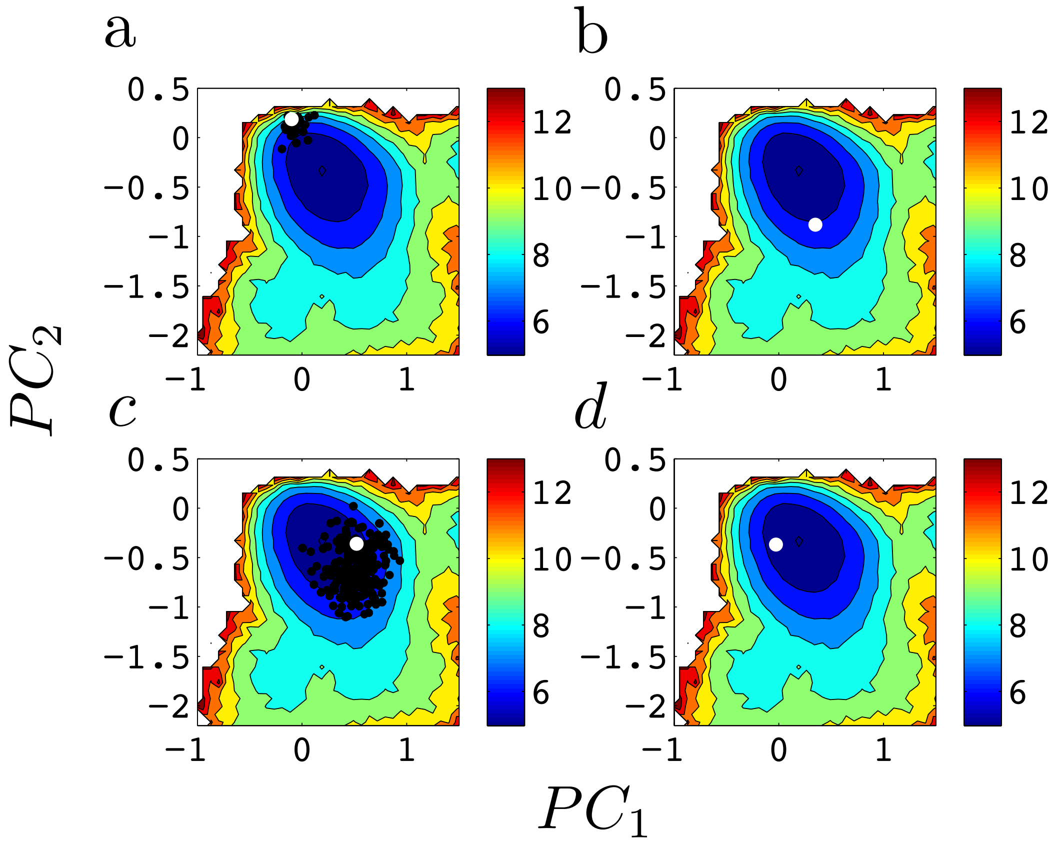


Figure S9: Panels a-d depict viral quasispecies in four randomly chosen individuals in the presence of immune pressure. These four cases correspond to different patterns of immune pressure. In each panel, every unique strain within the quasispecies is represented by a black dot at its location on the landscape and the corresponding consensus strain is marked with a large white dot. Due to the presence of diverse immune responses in a population, the quasispecies explore different regions of the fitness landscape in different infected hosts. Accordingly, the location of the corresponding consensus/dominant strain also explores the sequence space. The examples a-d also reflect the large variations in quasispecies diversity across individuals. In panels a and c, the immune pressure is such that mutation-selection balance results in a diverse quasispecies with many mutant strains. In contrast, Panels b and d are examples of cases where a restrictive pattern of immune pressure selects for a singular viral strain that dominates the entire quasispecies.

# 7 Comparison of the 3-body mutational probabilities computed from the population ensemble with intrinsic values

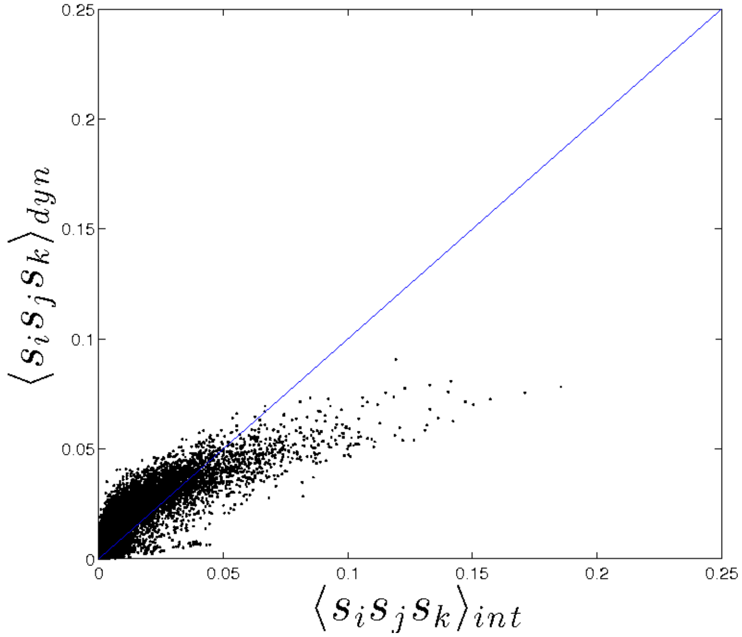


Figure S10: Comparison of 3-body mutational probabilities computed from the population ensemble resulting from quasispecies simulations at $\mu = 5 \times 10^{-3}$ with the corresponding values computed from MC sampling of $H_{int}[\vec{s}]$

## References


[1] Metropolis, N., Rosenbluth, A. W., Rosenbluth, M. N., Teller, A.H., and Teller, E. Equation of state calculations by fast computing machines. The Journal of Chemical Physics, 21:1087, 1953.

[2] Bishop, C. M. *Pattern Recognition and Machine Learning.* Springer New York, 2006.

[3] Friedman, J., Hastie, T., and Tibshirani, R. *The Elements of Statistical Learning.* Springer Series in Statistics, 2001.

[4] Van der Maaten, L. J. P., Postma, E. O., and Van den Herik, H. J. Dimensionality reduction: A comparative review. *Journal of Machine Learning Research*, 10:1–41, 2009.

[5] Los Alamos HIV Sequence Database. `http://www.hiv.lanl.gov/`.

[6] Ferguson, A. L. et al. Translating HIV sequences into quantitative fitness landscapes predicts viral vulnerabilities for rational immunogen design. Immunity, 38(3):606–617, 2013.

[7] Streeck, H. et al. Human immunodeficiency virus type 1-specific CD8+ T-cell responses during primary infection are major determinants of the viral set point and loss of CD4+ T cells. Journal of Virology, 83(15):7641–7648, 2009.

[8] F. F. Gonzalez-Galarza, Christmas, S., Middleton, D., and Jones, A. R. Allele frequency net: a database and online repository for immune gene frequencies in worldwide populations. Nucleic acids research, 39(suppl 1):D913–D919, 2011.

[9] p17 Epitope Map. `http://www.hiv.lanl.gov/content/immunology/maps/ctl/p17.html`.

[10] Eigen, M. Selforganization of matter and the evolution of biological macromolecules. Naturwissenschaften, 58(10):465–523, 1971.

[11] Kushal Tripathi, Rajesh Balagam, Nisheeth K Vishnoi, and Narendra M Dixit. Stochastic simulations suggest that hiv-1 survives close to its error threshold. *PLoS Computational Biology*, 8(9):e1002684, 2012.

[12] Feynman, R. P. and Hibbs, A. R. *Quantum Mechanics and Path integrals.* MacGraw Hill, 1965.
